# Supplementary material for: Learning from Web Data with Self-Organizing Memory Module
Source: arXiv:1906.12028 ancillary file (2020-03-11)
Supplement: Supplementary file 1 [file supplementary.pdf]

# Supplementary for
# Learning from Web Data with Self-Organizing Memory Module


Yi Tu, Li Niu*, Junjie Chen, Dawei Cheng, and Liqing Zhang*
MoE Key Lab of Artificial Intelligence, Department of Computer Science and Engineering
Shanghai Jiao Tong University, Shanghai, China
{tuyi1991,ustcnewly,chen.bys,dawei.cheng}@sjtu.edu.cn, zhang-lq@cs.sjtu.edu.cn


## 1. Proof and More Details of Value Slots

We first prove that $d_{y,l}$ and $r_{y,l}$ will approximate $\tilde{d}_{y,l}$ and $\tilde{r}_{y,l}$ by using $\mathcal{L}_{\text{d-value}}$ and $\mathcal{L}_{\text{r-value}}$ as the loss function. Recall that $\mathcal{S}$ denotes the whole training set and $\mathcal{B} \in \mathcal{S}$ is a training bag from the $y$-th category. $\bar{\mathbf{x}}$ is the bag-level feature and $\mathbf{y}$ is the one-hot vector of $y$. To distinguish the winner key slot of different bags, we use win($\bar{\mathbf{x}}$), instead of $z$, to denote the winner key slot index of $\bar{\mathbf{x}}$.

We first divide the d-value loss into $L$ separate parts for each d-value slot:

$$\begin{aligned} \mathcal{L}_{\text{d-value}} &= -\sum_{\mathcal{B}\in\mathcal{S}} \cos(\mathbf{y}, \mathbf{d}_z) & (1)\\ &= \sum_{l=1}^{L}\left(-\sum_{\mathcal{B}\in\mathcal{S}}\{\cos(\mathbf{y}, \mathbf{d}_l)|\text{win}(\bar{\mathbf{x}}) = l\}\right), & (2)\\ \text{s.t.} \quad & \|\mathbf{d}_l\|_1 = 1,\ \mathbf{d}_l \geq \mathbf{0},\ \forall\, l. & (3) \end{aligned}$$

We use $\mathcal{L}(\mathbf{d}_l) = -\sum_{\mathcal{B}\in\mathcal{S}}\{\cos(\mathbf{y}, \mathbf{d}_l)|\text{win}(\bar{\mathbf{x}}) = l\}$ to denote the corresponding loss term of $\mathbf{d}_l$. We can find that $\mathbf{d}_l$ is only influenced by the labels of the bags whose winner key slot is $\mathbf{k}_l$. Recall that $n_{y,l}$ denotes the number of training bags from the $y$-th category with winner key slot as $\mathbf{k}_l$. Then we can calculate $\mathcal{L}(\mathbf{d}_l)$:

$$\begin{aligned} \mathcal{L}(\mathbf{d}_l) &= -\sum_{y=1}^{C} n_{y,l}\cdot\cos(\mathbf{y}, \mathbf{d}_l) \\ &= -\sum_{y=1}^{C} n_{y,l}\cdot\frac{\mathbf{y}^T\mathbf{d}_l}{\|\mathbf{y}\|_2\|\mathbf{d}_l\|_2} \\ &= -\sum_{y=1}^{C} n_{y,l}\cdot\frac{d_{y,l}}{\|\mathbf{d}_l\|_2}. \end{aligned} \tag{4}$$

According to the Cauchy inequality theorem, we have:

$$\begin{aligned} \mathcal{L}(\mathbf{d}_l) &\geq -\left(\sum_{y=1}^{C}(n_{y,l})^2\sum_{y=1}^{C}\left(\frac{d_{y,l}}{\|\mathbf{d}_l\|_2}\right)^2\right)^{\frac{1}{2}} \\ &= -\left(\sum_{y=1}^{C}(n_{y,l})^2\right)^{\frac{1}{2}}, \end{aligned} \tag{5}$$

where the minimum condition is:

$$n_{y_1,l}\cdot\frac{d_{y_2,l}}{\|\mathbf{d}_l\|_2} = n_{y_2,l}\cdot\frac{d_{y_1,l}}{\|\mathbf{d}_l\|_2},\ \forall\, y_1, y_2. \tag{6}$$

Using the constraints in (3), the condition is equivalent to:

$$d_{y,l} = \frac{n_{y,l}}{\sum_{y=1}^{C} n_{y,l}} = \tilde{d}_{y,l}\ ,\forall\, y. \tag{7}$$

So far, we have proved that the minimum of $\mathcal{L}(\mathbf{d}_l)$ can be reached when $d_{y,l} = \tilde{d}_{y,l},\ \forall\, y$ . Similarly, we can prove that the minimum of the loss term $\mathcal{L}_{\text{r-value}}$ for $\mathbf{r}_y$ can be reached when $r_{y,l} = \tilde{r}_{y,l},\ \forall\, l$ . During training, we use the gradient descent algorithm to optimize $\mathbf{d}_l$ and $\mathbf{r}_y$ to achieve the minimum of $\mathcal{L}_{\text{d-value}}$ and $\mathcal{L}_{\text{r-value}}$. Notice that these two optimization tasks are both convex optimization problem, so we can efficiently approximate the minimal loss and the minimum condition.

To satisfy the constraints in (3), we first construct two auxiliary matrices $\mathbf{D}^{'} \in \mathcal{R}^{C\times L}$ and $\mathbf{R}^{'} \in \mathcal{R}^{C\times L}$. They are not constrained and can be directly optimized by gradient descent. Then we obtain the the desired $\mathbf{D}$ and $\mathbf{R}$ with softmax normalization:

$$\begin{aligned} d_{y,l} &= \frac{\exp(d^{'}_{y,l})}{\sum_{y=1}^{C}\exp(d^{'}_{y,l})}, \\ r_{y,l} &= \frac{\exp(r^{'}_{y,l})}{\sum_{l=1}^{L}\exp(r^{'}_{y,l})}, \end{aligned} \tag{8}$$

where the constraints in (3) are satisfied.


*Corresponding author.

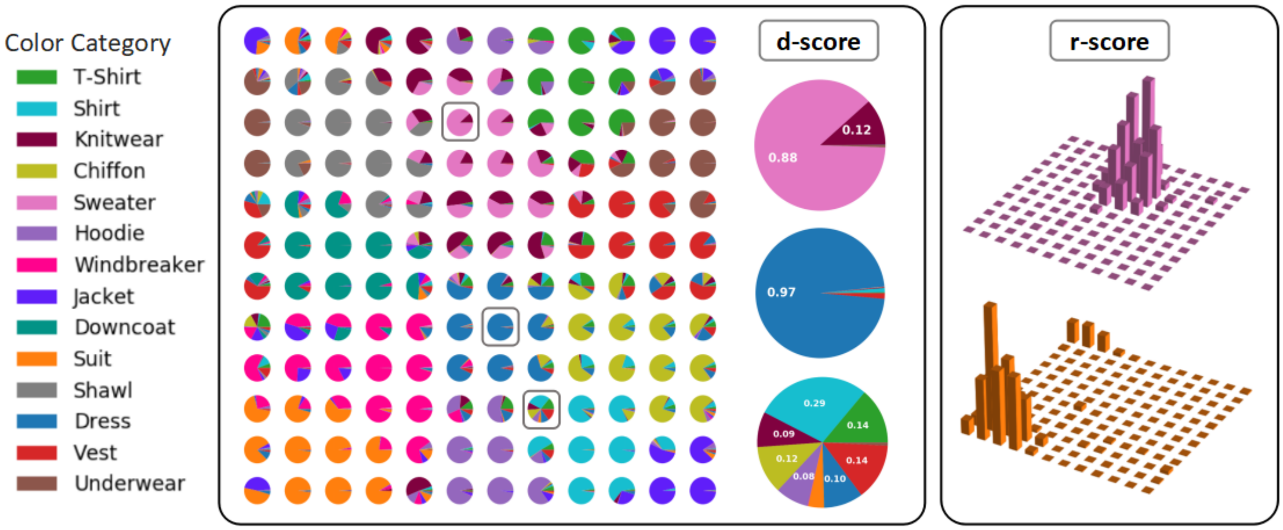


Figure 1. Illustration of the memory module results on the Clothing1M dataset. **Left:** Pie charts of d-scores of all key slots. We choose three slots to show the detailed d-scores for each category. The first two have a high d-score for "Sweater" and "Dress" respectively, while the third one has a low d-score for any category. **Right:** Bar charts of r-scores of all key slots for "Sweater" and "Suit".

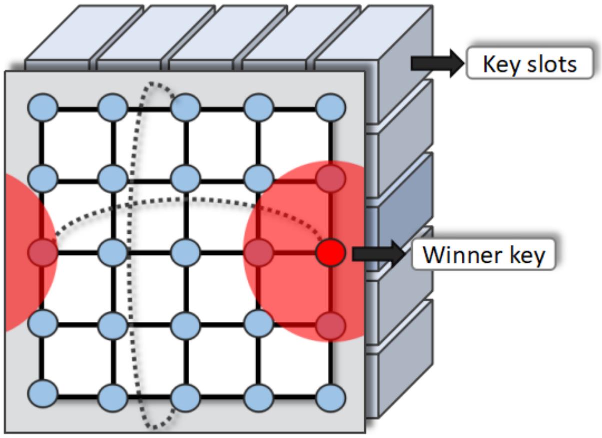


Figure 2. A $5 \times 5$ square grid with $L = 25$ key slots. Dashed lines denote two extra edges. The red cell is the winner key $\mathbf{k}_z$ of a given input sample, and the pink circle denotes its neighborhood $\mathtt{N}(\mathbf{k}_z, \delta)$ within the radius $\delta$=1.

## 2. More Details of the Memory Module

In the self-organizing memory module, we arrange the key slots on a $5 \times 5$ square grid. In order to ensure that all key slots are spatially equivalent and have the same number of neighbors, we connect the key slots on the edges to their imaginary neighbors with extra edges as illustrated in Figure 2. For an example, based on 2D indices of cells in a $5 \times 5$ square grid, we use $((i_1, j_1), (i_2, j_2))$ to denote an edge between cell $(i_1, j_1)$ and cell $(i_2, j_2)$. Then, the extra edges are $\{((i, 1), (i, L))|i = 1, 2, ..., 5\}$ and $\{((1, i), (L, i))|i = 1, 2, ..., 5\}$, which means that the grid is left-right connected and top-bottom connected.

Based on the architecture defined above, each key slot has its spatial neighbors. When updating the winner key slot, we also update its spatial neighbors. There are two advantages of applying such a neighborhood constraint:

1) The key slots will be less sensitive to initialization. Given any initialization, since we will always update a winner key slot and its neighbor slots, the whole key slots will surely overlap with the feature space of the bag-level features after enough iterations.

2) The clustering results will be more balanced. For any frequently visited key slot which usually implies a dense cluster, its visits will propagate to its neighboring key slots, so that any dense cluster will be split into several small clusters captured by multiple key slots.

## 3. More Visualization Results of the Memory Module

To demonstrate the effectiveness of our memory module, we illustrate the learned d-scores and r-scores of all $L = 144$ key slots on Clothing1M in Figure 1, in which 14 colors denote 14 categories. For d-score, each pie chart shows the d-scores of one key slot for all 14 categories. For r-score, each bar chart shows the r-scores of all key slots on a particular category.

## 4. More Details of K-means Baseline

We have a baseline named SOMNet+K-means in Table 1 in the main text, which means that we use K-means algorithm to replace the self-organizing memory module for clustering. Since K-means cannot be trained with our network in an end-to-end manner, we run it after each training

epoch.

Following the setting of the memory module, we set the same number of clustering centers when using K-means method. We treat each clustering center as a key slot like in the memory module. After clustering, we calculate $\tilde{d}_{y,l}$ and $\tilde{r}_{y,l}$ from the clustering results and use them as the d-score and r-score for ROI selection.
